# Supplementary material for: One Metric to Measure them All: Localisation Recall Precision (LRP) for Evaluating Visual Detection Tasks
Source: arXiv:2011.10772 source file (2021-11-21)
Supplement: Supplementary file 1 [file 0.FrequentlyUsedTerms.tex]

\section{Frequently Used Terms and Notation}
\label{sec:DefNot}
%In the following, we first present the definitions and notation used throughout the paper, and formally define the tasks that we consider. 

%\subsection{Frequently Used Terms and Notation}
Table \ref{tab:notation} presents the notation used throughout the paper, and below is a list of frequently used terms.
\begin{table}
\centering
\caption{Frequently used notations in the paper. \label{tab:notation}}
\footnotesize
    \begin{tabular}{|>{\centering\arraybackslash}m{.15\linewidth}|>{\centering\arraybackslash}m{.7\linewidth}|}
         \hline
         \textbf{Symbol} &\textbf{Denotes} \\ \hline
         $\mathrm{AP^C}$&COCO-Style AP\\ \hline
         $\mathrm{AP}_\tau$&AP when the TPs are validated from the $\mathrm{lq}(\cdot,\cdot)$ threshold of $\tau$\\ \hline
%         $B$&A bounding box\\ \hline
%         $c$&A class label\\ \hline
%         $\mathcal{C}$&The set of class labels in the dataset\\ \hline
         $d$&A detection such that $d \in \mathcal{D}$ \\ \hline
         $d_g$&A TP detection that matches ground truth $g$ and qualifies for performance evaluation\\ \hline
         $\mathcal{D}$&A set of detections\\ \hline
%         $\mathcal{D}_s$&A set of detections thresholded from confidence score $s$\\ \hline
         FN&False Negative\\ \hline
         FP&False Positive\\ \hline
         $g$&A ground truth such that $g \in \mathcal{G}$ \\ \hline
         $\mathcal{G}$&A set of ground truths\\ \hline
%         $\mathrm{IoU}(\cdot, \cdot)$&Intersection over Union of two polygons\\ \hline
%         $\mathrm{IoU_B}(\cdot, \cdot)$&IoU of two bounding boxes\\ \hline
%         $\mathrm{IoU_M}(\cdot, \cdot)$&IoU of two segmentation masks\\ \hline
%         $k$&A single keypoint\\ \hline
%         $K$&A set of keypoints\\ \hline
         $\mathrm{lq}(\cdot, \cdot)$&A localisation quality function. (e.g. $\mathrm{IoU_B}(\cdot, \cdot)$) \\ \hline
%         $M$&A segmentation mask\\ \hline
         $\mathrm{N_{FN}}$&Number of FNs\\ \hline
         $\mathrm{N_{FP}}$&Number of FPs\\ \hline
         $\mathrm{N_{TP}}$&Number of TPs\\ \hline
%         $\mathrm{OKS}(\cdot, \cdot)$&Similarity between two sets of object keypoints\\ \hline
%         $s$&A confidence score\\ \hline
         $s^*$&LRP-Optimal confidence score\\ \hline
%         $\mathcal{S}$&A set of confidence scores\\ \hline
         TP&True Positive\\ \hline
         $\tau$&TP validation threshold in terms of localisation quality\\ \hline
%         $|| \cdot - \cdot||$&Euclidean distance \\ \hline
         
    \end{tabular}
\end{table}

\noindent \textbf{Hard Prediction:} A type of visual object detector output which identifies each object with (i) a set of identifiers to locate an object (e.g. bounding box, mask, keypoints), and (ii) its class label.

\noindent \textbf{Soft Prediction:} A type of visual object detector output which identifies each object with (i) a set of identifiers to locate an object (e.g. bounding box, mask, keypoints), (ii) its class label and (iii) the confidence score of the prediction.
 
\noindent \textbf{Bounding Box:} A rectangle on the image. Formally, a bounding box, denoted by $B$, is generally represented by $[x_1,y_1,x_2,y_2]$ with  $(x_1,y_1)$ denoting the top-left corner and  $(x_2,y_2)$ the bottom-right corner, with the constraints $x_2>x_1$ and $y_2>y_1$. 

\noindent \textbf{Keypoint Set:} A set of coordinates to represent an object on the image such that each element is a two tuple $(x_i, y_i)$ identifying a keypoint of an object. 

\noindent \textbf{Segmentation Mask:} A set of pixels presenting which pixels belong to a particular object. 

\noindent \textbf{Intersection Over Union (IoU):} For two polygons $P_g$ and $P_d$, Intersection over Union (IoU) \cite{PASCAL,ImageNet}, $\mathrm{IoU}(P_g,P_d)$ is defined as :
\begin{align}
\label{eq:IoU}
\mathrm{IoU}(P_g,P_d)&=\frac{\mathrm{A}(P_g \cap P_d)}{\mathrm{A}(P_g \cup P_d)},
\end{align}
where $\mathrm{A}(P)$ is the area of the polygon $P$ (i.e. number of pixels delimited by $P$). These polygons are represented by bounding boxes for object detection, and by masks for segmentation tasks (e.g. instance segmentation, panoptic segmentation). $\mathrm{IoU} \in [0,1]$ and it is used to evaluate the localisation quality of a detection bounding box/mask with respect to its ground truth box/mask.

\noindent \textbf{Object Keypoint Similarity (OKS):} Given target and estimated keypoint sets, $K_g$ and $K_d$ respectively, with $k_g^i \in K_g$ and $k_d^i \in K_d$ being the $i$th keypoint of the object represented by a 2D coordinate on the image, Object Keypoint Similarity (OKS) \cite{COCO} between $k_g^i$ and $k_d^i$, denoted by $\mathrm{OKS}(k_g^i,k_d^i)$, is
\begin{align}
\label{eq:OKSSingle}
\mathrm{OKS}(k_g^i,k_d^i) =  \frac{ \exp(-||k_g^i- k_d^i||^2)}{2 (S \kappa^i)^2},
\end{align}
where $|| \cdot - \cdot||$ is Euclidean distance, $\kappa^i$ is the constant corresponding to $i$th keypoint to control falloff, and $S$ is the object scale (e.g. the area of the ground truth bounding box divided by the total image area). Then, OKS between $K_g$ and $K_d$, $\mathrm{OKS}(K_g,K_d)$, is simply the average of $\mathrm{OKS}(k_g^i,k_d^i)$ over single keypoints annotated in the dataset:
\begin{align}
\label{eq:OKS}
\mathrm{OKS}(K_g,K_d) =  \frac{ 1}{|K_g|}\sum \limits_{i \in |K_g|} \mathrm{OKS}(k_g^i,k_d^i).
\end{align}
Similar to $\mathrm{IoU}(\cdot,\cdot)$; $\mathrm{OKS}(\cdot,\cdot) \in [0,1]$ and a larger $\mathrm{OKS}(\cdot,\cdot)$ implies better localisation quality.

%\noindent \textbf{Performance Measure:} A function that is used to evaluate the performance of a task. 

%\noindent \textbf{Performance Metric:} A performance measure that is proven to satisfy the metricity conditions: reflexivity, symmetry and triangle inequality.

\blockcomment{
\subsection{Formal Definitions of the Detection Tasks Considered in this Paper}
In this paper, we consider the following four detection tasks (see \figref{\ref{fig:tasks}}):

\noindent \textbf{Object Detection:} The aim of the object detection is to identify and localize all the objects in an image using bounding boxes. Accordingly, the output of an object detector consists of tuples $d=\{B, c, s\}$. 

\noindent \textbf{Keypoint Detection:} The aim of the keypoint detection is to identify the objects along with their keypoints. A common example is human pose estimation, in which 17 keypoints are expected to determined by the detector. For such class-specific detectors, only the keypoints are expected to be reported. From a generic keypoint detection perspective, the output of a keypoint detector consists of tuples $d=\{K, c, s\}$.

\noindent \textbf{Instance Segmentation:} The aim of the instance segmentation is to identify and localize all the objects in an image using segmentation masks. Accordingly, the output of a detector consists of tuples $d=\{M, c, s\}$.

\noindent \textbf{Panoptic Segmentation:} The aim of the panoptic segmentation is to identify and localize all the objects also by classifying the background. In such a way it combines semantic segmentation task with the instance segmentation task. Accordingly, the output of a detector consists of tuples $d=\{M, c\}$.
}
