# Supplementary material for: One Metric to Measure them All: Localisation Recall Precision (LRP) for Evaluating Visual Detection Tasks
Source: arXiv:2011.10772 source file (2021-11-21)
Supplement: Supplementary file 6 [file 5.PQLRPSimilarityDerivation.tex]

\section{The Similarity between PQ and LRP Errors}
\label{app:similarity}
In this section, we derive \equref{\ref{eq:PQvsLRP}}: 
\begin{align}
        \label{eq:PQvsLRP2}
        1 -\mathrm{PQ} =  \frac{1}{\hat{Z}} \left( \sum \limits_{i=1}^{\mathrm{N_{TP}}}  \frac{1-\mathrm{lq}(g_i, d_{g_i})}{1-0.50}+\mathrm{N_{FP}} +\mathrm{N_{FN}} \right) ,
\end{align}
where $\hat{Z} = {\textcolor{red}{2} \mathrm{N_{TP}}+\mathrm{N_{FP}} +\mathrm{N_{FN}}}$. LRP and PQ Errors are very similar:  Removing $2$ (in red) from $\hat{Z}$ yields $1-\mathrm{PQ} = \mathrm{LRP}$. 

Recall from \equref{\ref{eq:PQ}} that PQ is defined as (see Table \ref{tab:notation} for the notation):
\begin{align}
\label{eq:PQ_}
\mathrm{PQ}(\mathcal{G},\mathcal{D}) = \frac{1 }{{\mathrm{N_{TP}}+ \frac{1}{2} \mathrm{N_{FP}} + \mathrm{\frac{1}{2} N_{FN}}}} \left( \sum \limits_{i=1}^{\mathrm{N_{TP}}} \mathrm{IoU}(g_i, d_{g_i}) \right).
\end{align}
First, we replace $\mathrm{IoU}(\cdot, \cdot)$ in \equref{\ref{eq:PQ_}} by $\mathrm{lq}(\cdot, \cdot)$ to align the definitions of LRP and PQ:
\begin{align}
\label{eq:PQ2}
\mathrm{PQ}(\mathcal{G},\mathcal{D}) = \frac{1 }{{\mathrm{N_{TP}}+ \frac{1}{2} \mathrm{N_{FP}} + \mathrm{\frac{1}{2} N_{FN}}}} \left( \sum \limits_{i=1}^{\mathrm{N_{TP}}} \mathrm{lq}(g_i, d_{g_i}) \right).
\end{align}
Then, just by simple algebraic operations, we manipulate \equref{\ref{eq:PQ2}}:
\begin{align}
    \mathrm{PQ} &= 1 - 1 + \frac{\sum \limits_{i=1}^{\mathrm{N_{TP}}} \mathrm{lq}(g_i, d_{g_i}) }{\mathrm{N_{TP}} + \frac{1}{2} \mathrm{N_{FP}}+ \frac{1}{2} \mathrm{N_{FN}}} \\
    &= 1 - \left( 1 - \frac{\sum \limits_{i=1}^{\mathrm{N_{TP}}} \mathrm{lq}(g_i, d_{g_i}) }{\mathrm{N_{TP}} + \frac{1}{2} \mathrm{N_{FP}}+ \frac{1}{2} \mathrm{N_{FN}}} \right) \\
    &= 1 -  \frac{ \mathrm{N_{TP}} + \frac{1}{2} \mathrm{N_{FP}}+ \frac{1}{2} \mathrm{N_{FN}} - \sum \limits_{i=1}^{\mathrm{N_{TP}}} \mathrm{lq}(g_i, d_{g_i}) }{\mathrm{N_{TP}} + \frac{1}{2} \mathrm{N_{FP}}+ \frac{1}{2} \mathrm{N_{FN}}} \\
    &= 1 -  \frac{ \mathrm{N_{TP}}  - \sum \limits_{i=1}^{\mathrm{N_{TP}}} \mathrm{lq}(g_i, d_{g_i})+ \frac{1}{2} \mathrm{N_{FP}}+ \frac{1}{2} \mathrm{N_{FN}} }{\mathrm{N_{TP}} + \frac{1}{2} \mathrm{N_{FP}}+ \frac{1}{2} \mathrm{N_{FN}}}\\
    &= 1 -  \frac{ \sum \limits_{i=1}^{\mathrm{N_{TP}}} 1  - \sum \limits_{i=1}^{\mathrm{N_{TP}}} \mathrm{lq}(g_i, d_{g_i})+ \frac{1}{2} \mathrm{N_{FP}}+ \frac{1}{2} \mathrm{N_{FN}} }{\mathrm{N_{TP}} + \frac{1}{2} \mathrm{N_{FP}}+ \frac{1}{2} \mathrm{N_{FN}}} 
\end{align}
\begin{align}
    &= 1 -  \frac{ \sum \limits_{i=1}^{\mathrm{N_{TP}}} \left(1  - \mathrm{lq}(g_i, d_{g_i}) \right) + \frac{1}{2} \mathrm{N_{FP}}+ \frac{1}{2} \mathrm{N_{FN}} }{\mathrm{N_{TP}} + \frac{1}{2} \mathrm{N_{FP}}+ \frac{1}{2} \mathrm{N_{FN}}} \\
    \label{eq:PQfinal}
    &=1 -  \frac{1}{\hat{Z}} \left( \sum \limits_{i=1}^{\mathrm{N_{TP}}}  \frac{1-\mathrm{lq}(g_i, d_{g_i})}{1-0.50}+\mathrm{N_{FP}} +\mathrm{N_{FN}} \right),
\end{align}
where $\hat{Z} = {\textcolor{red}{2} \mathrm{N_{TP}}+\mathrm{N_{FP}} +\mathrm{N_{FN}}}$. As a result, we can rewrite \equref{\ref{eq:PQfinal}} to express the PQ Error (i.e. 1-PQ) as follows:
\begin{align}
    1-\mathrm{PQ}= \frac{1}{\hat{Z}} \left( \sum \limits_{i=1}^{\mathrm{N_{TP}}}  \frac{1-\mathrm{lq}(g_i, d_{g_i})}{1-0.50}+\mathrm{N_{FP}} +\mathrm{N_{FN}} \right)
\end{align}
